# Supplementary material for: Rethinking Network Pruning -- under the Pre-train and Fine-tune Paradigm
Source: arXiv:2104.08682 source file (2022-01-16)
Supplement: Supplementary file 1 [file appendix.tex]

\section{Appendix}
\label{sec:app}

This is an appendix.
